# Supplementary material for: Structured flows regulate droplet dynamics in phase-separating fluids
Source: arXiv:2407.02792 source file (2026-09-11)
Supplement: Supplementary file 1 [file supplement.tex]

\documentclass[aps,pre,onecolumn,superscriptaddress,article,12pt]{revtex4-2}
\usepackage{amsmath}
\usepackage{amsfonts}
\usepackage{graphicx}
\usepackage[subpreambles=true]{standalone}
%\usepackage{tikz-feynman}
%\usepackage{cancel}
%\usepackage[numbers,sort&compress]{natbib}

%\addbibresource{flow_driven_phase_separation.bib}

\usepackage[colorinlistoftodos,prependcaption,textsize=small]{todonotes}
\usepackage{color}
\definecolor{red}{rgb}{0.75,0,0}
\definecolor{blue}{rgb}{0,0,0.75}
\definecolor{green}{rgb}{0,0.5,0}

\makeatletter

\newcommand{\eq}{\begin{equation}}
\newcommand{\eeq}{\end{equation}}
\newcommand{\aeq}{\begin{equation}\begin{aligned}}
\newcommand{\eaeq}{\end{aligned}\end{equation}}

\makeatother

\begin{document}
\title{Supplemental materials to manipulating liquid-liquid phase separation using patterned flow}

\author{Yulin Li}
\thanks{These authors contributed equally}
\affiliation{Fujian Provincial Key Laboratory for Soft Functional Materials Research, Research Institute for Biomimetics and Soft Matter, Department of Physics, Xiamen University, Xiamen, Fujian 361005, China}

\author{Tong Zhou} 
\thanks{These authors contributed equally}
\affiliation{Fujian Provincial Key Laboratory for Soft Functional Materials Research, Research Institute for Biomimetics and Soft Matter, Department of Physics, Xiamen University, Xiamen, Fujian 361005, China}
 
\author{Yanyu Li}
\thanks{These authors contributed equally}
\affiliation{Fujian Provincial Key Laboratory for Soft Functional Materials Research, Research Institute for Biomimetics and Soft Matter, Department of Physics, Xiamen University, Xiamen, Fujian 361005, China}

\author{Qi Zhang}
\affiliation{School of Science, Jiangsu University of Science and Technology, Zhenjiang, Jiangsu 212100, China}

\author{Zhihong You}
\thanks{Corresponding author: zhyou@xmu.edu.cn}
\affiliation{Fujian Provincial Key Laboratory for Soft Functional Materials Research, Research Institute for Biomimetics and Soft Matter, Department of Physics, Xiamen University, Xiamen, Fujian 361005, China}
	
\date{\today}
	
\maketitle

% ===============================================

\section{Numerical implementations}
This section introduces the detailed numerical implementations, including the numerical solver of Eq. (1) in the main text and the overall procedure to generate structured flow fields.

The first step is to construct a structured flow field with the condition of incompressibility. To do this, we use the vortex-stream function method~\cite{barragy1997stream}. Specifically, we first prescribe a velocity field with an expected spatial structure $\textbf{v}_0$, which usually does not satisfy the condition of incompressibility. To enforce incompressibility, we calculate the vorticity field of $\textbf{v}_0$ using $\omega=\hat{z}\cdot \nabla\times\textbf{v}_0$, and then get the stream function $\psi$ of $\omega$ by solving the Poison equation $\nabla^2\psi=-\omega$. Finally, by setting $v_x=\partial_y\psi$ and $v_y=-\partial_x\psi$, we obtain a velocity field $\textbf{v}=(v_x, v_y)$ which has a very similar structure as $\textbf{v}_0$ but is also incompressible. The specific $\textbf{v}_0$ used to construct each flow can be found in Sec. 6. 

Upon given the prescribed flow field, Eq. (1) can be solved numerically using the finite difference method. For simplicity, we consider a square periodic box of size $L\times L$ throughout the paper. Space is discretized into uniform square grids of size $h$ using a forth-order central difference scheme. To integrate in time, we use the Runge–Kutta–Chebyshev scheme with a time step $\Delta t$, which provides enhanced numerical stability and allows for a large time step \cite{verwer1990convergence}. Rescaled units (see the main text) are used by default. Numerically, this is done by setting: $a=1, k=1$ and $M=1$. The space and time steps are $h=1$ and $\Delta t=1$, and the system size is $L=128$, unless otherwise specified.

The initial condition of phase field $\phi$ is either set as a circular droplet or, a uniform field with a mean value $\phi_0$ perturbed with a very small random noise. In the former case, we set $\phi(\textbf{r})=(\text{tanh}(r_0 - \Delta r)+1)/2$, which gives a circular droplet with radius $r_0$ and an interface width $1$, where  $\Delta r = |\textbf{r}-\textbf{r}_c|$ and $\textbf{r}_c$ is the center of droplet. For a uniform phase field, $\phi_0$ represents the composition of the fluid mixture.

% ----------------------------------------------
\section{Quantifying the area and position of droplets}

Since the average $\phi$ is no more than $0.5$ in this article, the lessor phase, with $\phi=1$, usually nucleates in the form of droplets, immersed in the background phase with $\phi=0$, see e.g. Fig. 1a in the main text. The area of each droplet is then the total area of interconnected grid points with $\phi\ge 0.5$. The mean area of droplets is calculated using $\langle A\rangle=\sum_j A_j^2/\sum_j A_j$, where $A_j$ is the area of the $j$th droplet. Note that each droplet is weighted by its area here.

When it comes to the center of mass, the system usually has one droplet only. The center of mass $\textbf{R}_c=(X_c, Y_c)$ can thus be easy calculated using $X_c = (\sum_i x_i \phi_i ) / M$ and $Y_c = (\sum_i y_i \phi_i ) / M$. Here, $i$ is the index of grid point, summing over all grid points, and $M = \sum_i \phi_i $ is the total phase in the system.

% ---------------------------------------------
\section{Alignment of droplet interface to the flow streamline}

\begin{figure}[h]
    \centering
    \includegraphics[width=0.8\textwidth]{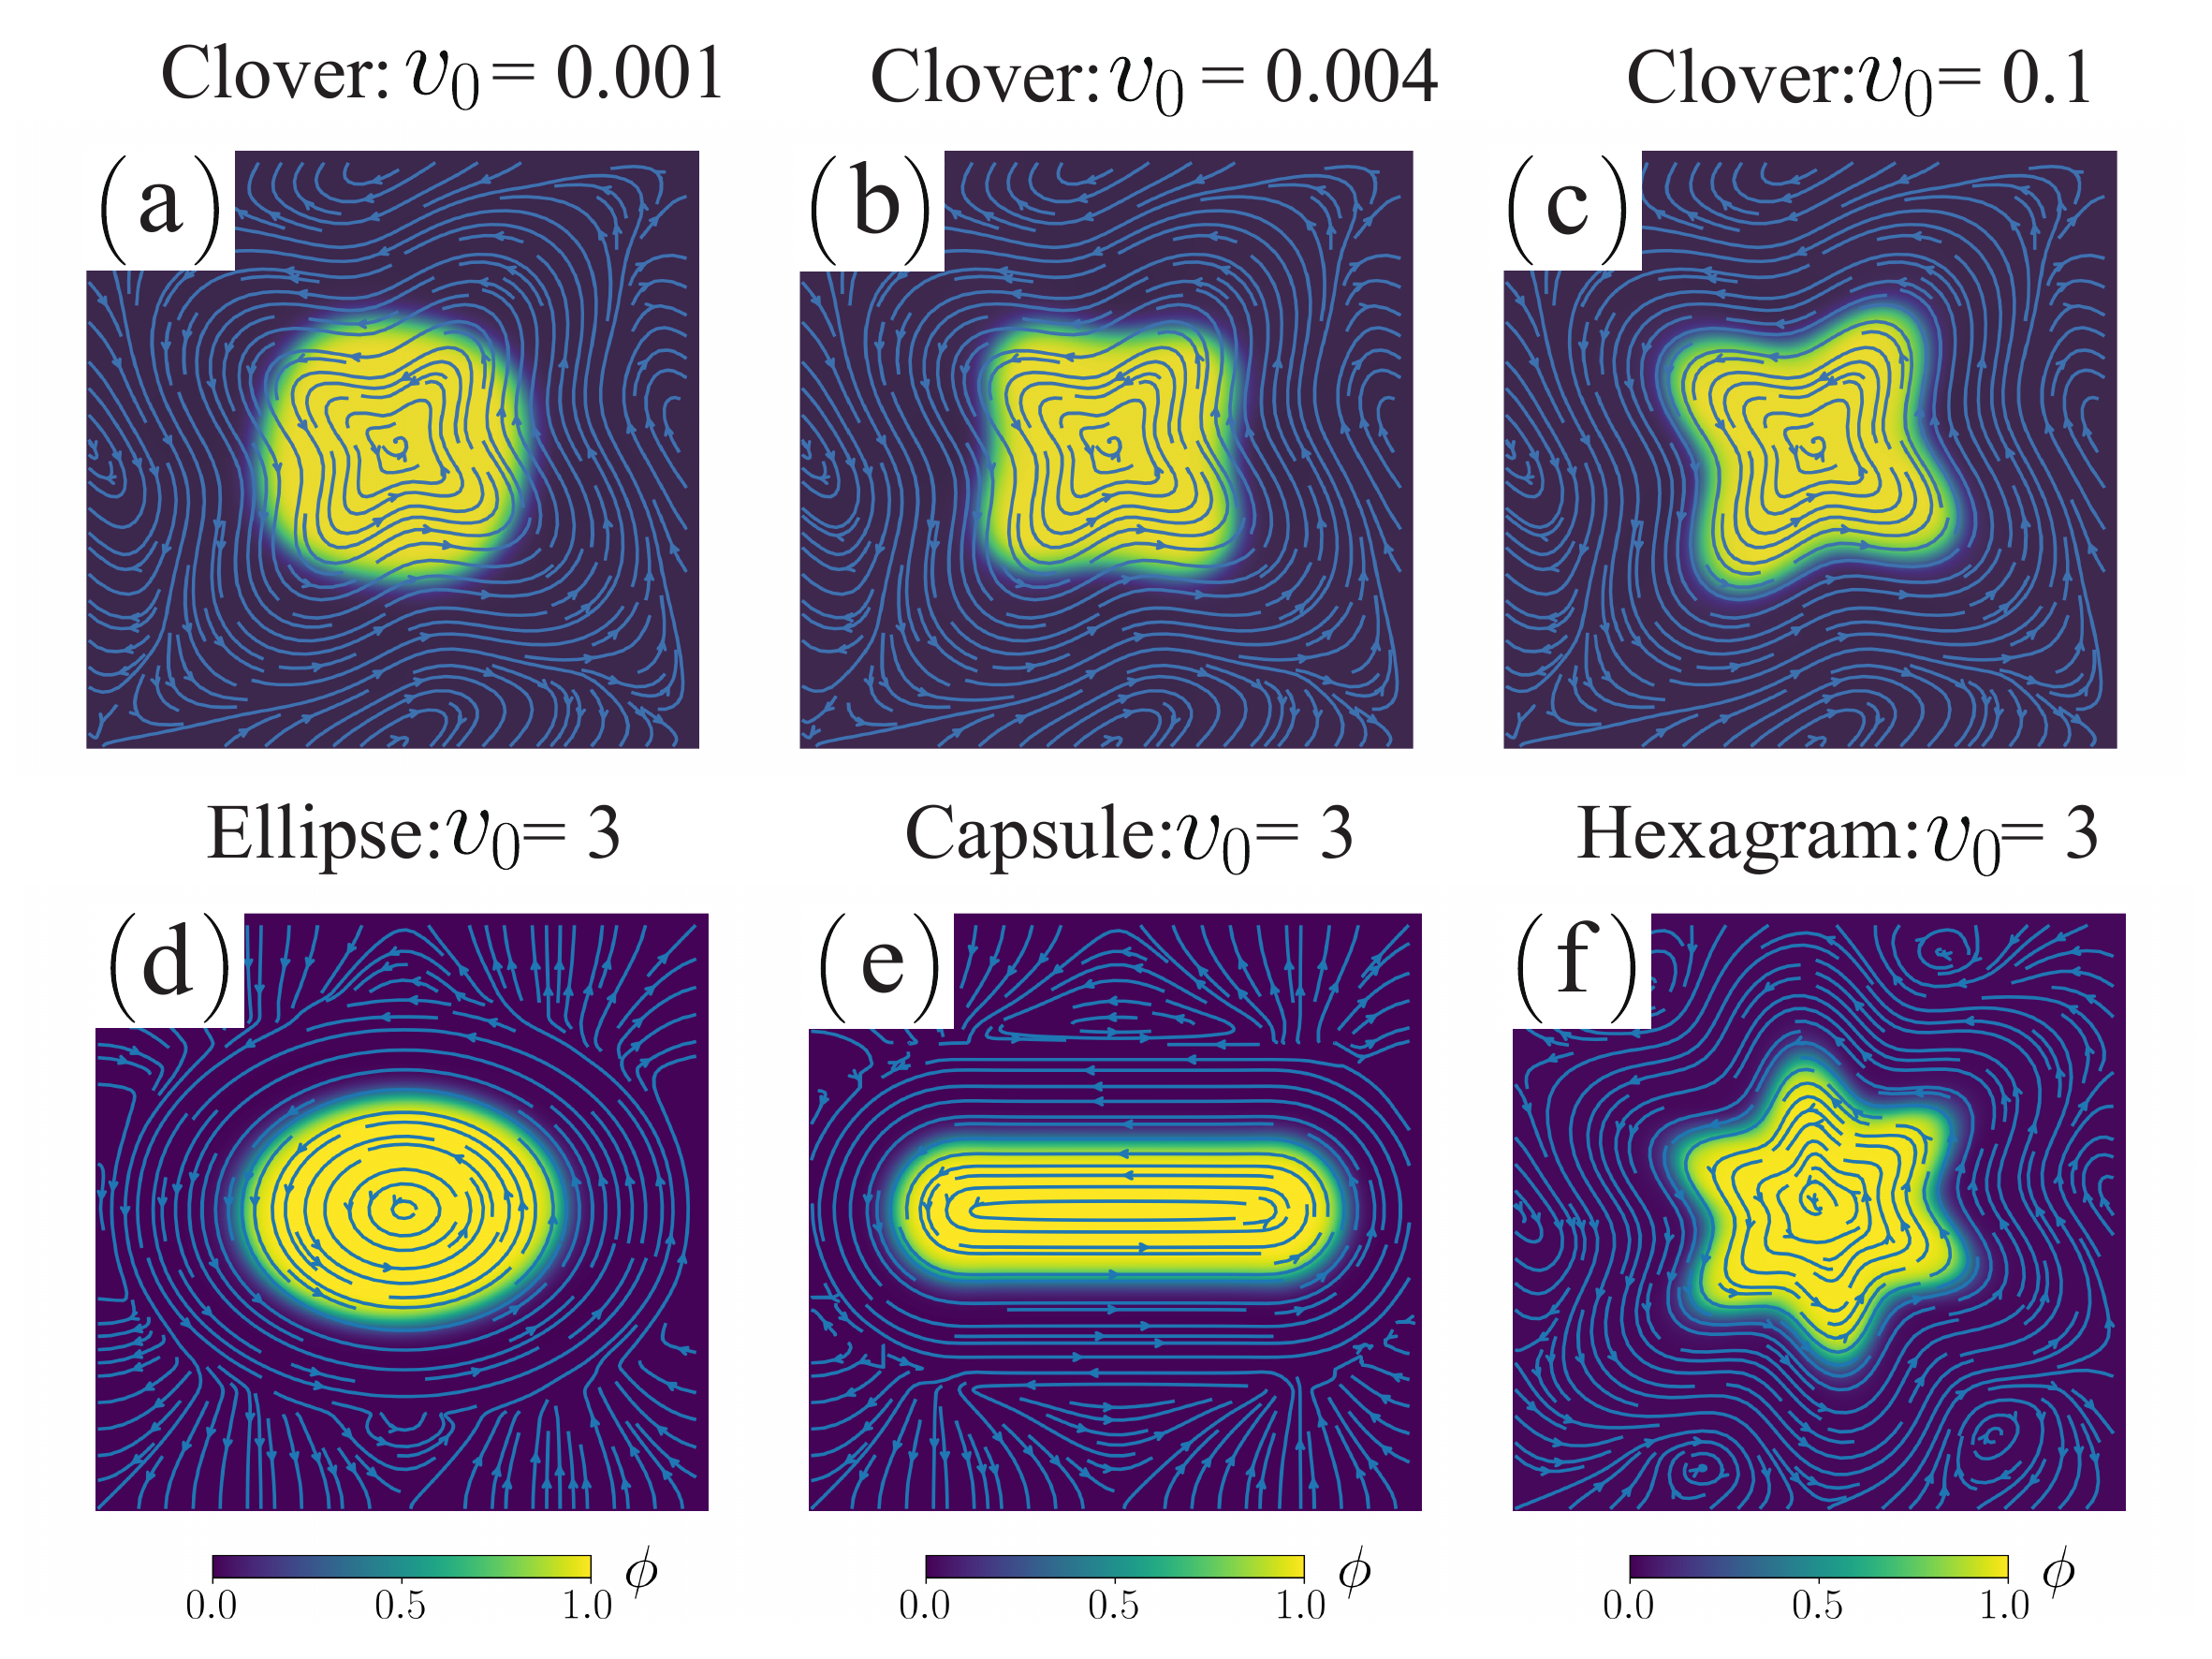}    
    \caption{Alignment of droplet interface to the flow streamline. (a-c) Steady shape of droplets in clover-shaped vortices with the same structure, but different overall speeds. (d-e) Steady shape of droplets in different structured vortices. The detailed vortex structures can be found in Sec. S6D.}
    \label{figS:align}
\end{figure}

When placed in a structured flow, the droplet interface tends to align parallelly to the flow streamline. The degree of alignment depends on the velocity gradient. As shown in Figs. \ref{figS:align}a-\ref{figS:align}c, stronger velocity gradient promotes better alignment to the streamline. This originates from the competition between interfacial tension and flow advection. On the one hand, advection by the flow tends to align the interface parallelly to the flow streamline. This is because an interface not parallel to the streamline will experience a net rotation by the shear flow, which only vanishes at parallel alignment. On the other hand, interfacial tension tends to restore the interface back to a circular geometry. Increasing the overall flow speed gives larger velocity gradients, thus enhancing the effect of alignment, see Figs. \ref{figS:align}a-\ref{figS:align}c. Figures \ref{figS:align}d-\ref{figS:align}f show shapes of droplets driven by flows with different structures.

% ----------------------------------------
\section{Constitutive relation and phase portrait}

In this section, we give some detailed discussion on the constitutive relation and phase portrait of droplets in structured vortices. Both are used to give quantitative predictions on droplet's behavior in structured vortices.

\subsection{Constitutive relation}
To give quantitative predictions on the size variation of droplets, it is necessary to know how their ECP's change with their sizes. This is very similar to the pressure-volume relation of the ideal gas: the droplet area is analogous to the gas volume which uniquely determines the state of the system, whereas the ECP plays the role of pressure which drives the change of state variable. Hence, we refer to the ECP-area relation as the constitutive relation of droplets in a structured vortex. 

The situation is slightly more complicated than ideal gas though. The chemical potential is highly inhomogeneous in a deformed droplet (see e.g. Fig. 1b and 2b), making it very difficult to measure the ECP directly from the chemical potential field. We thus resort to a more operational way of determining the ECP. Specifically, suppose a deformed droplet in vortex can stably coexist with a circular droplet not advected by flow. In that case, the chemical potential of the circular droplet, which is well-defined according to equilibrium thermodynamics, is considered to be ECP of the deformed droplet. In practice, we implant the vortex concerned at the lower-left corner of the simulation box, leaving the rest of system flowless. Then, we place a droplet of size $S$ in the given vortex, and another circular droplet in the top-right corner where the flow is negligible, see e.g. Fig. 2a in the main text. By gradually varying the initial area of the circular droplet, we can always find an area $S^*$ at which the two droplets have no exchange of mass. Repeating this procedure for different $S$ values, we finally have a set of $S-S^*$ correspondences. Interestingly, there is no need to determine the precise value of ECP's. This is because the chemical potential of a circular droplet decreases monotonically with increasing area. Hence, given two droplets each in a structured vortex, one can get the $S^*$ value of each droplet, and the one with larger $S^*$ value has a lower ECP, hence will increase in size over time. Consequently, the $S-S^*$ correspondence is the constitutive relation we need to predict the size variation of droplets.

We will briefly discuss the shape of $S-S^*$ curves in Fig. 2g in the main text. Note that the $S-S^*$ curve of a circular droplet is merely a straight line $S^*=S$. One immediately sees that the $S-S^*$ curves in Fig. 2g are way below the line $S^*=S$. This indicates that structured vortices can significantly decrease the value of $S^*$, thus increasing the ECP's of droplets by enforcing high curvatures at the droplet interface. In certain regions, the $S-S^*$ curve can even exhibit negative slopes, which means that a larger droplet has a higher ECP, the exact opposite of droplets at thermal equilibrium. It is the negative-slope regions that allow stable coexistence of droplets (see the section below). We want to point out that not all structured vortices can have such effects. A circular vortex, for example, cannot change the ECP of a droplet located at the vortex center. To create a negative slope in the $S-S^*$ curve, one needs to design a vortex structure such that the mean curvature of the droplet increases with its size. In other words, the larger the droplet, the pointier the corners. This also highlights the capability of structured vortices in remodeling the ECP landscape of droplets.

\subsection{Phase portrait}
Phase portrait is an important concept in the field of dynamical systems, which is used to analyze the global behavior of evolution trajectories in phase space~\cite{butkovskiy2012phase}. Mathematically, phase portrait is a geometric representation of orbits in phase space. Here, we use this concept to better visualize the overall behavior of droplet size variation.

As mentioned before, the area of a droplet can be used as a state variable. The state of a two-droplet system can be characterized by the combined $(S_1, S_2)$, where $1$ and $2$ are the indices of the two droplets, respectively. The time evolution of the system then corresponds to a trajectory in the two-dimensional phase space spanned by $S_1$ and $S_2$ (see e.g. dotted lines in Fig. 2h in the main text). To reveal the global behavior of the system, instead of showing all evolution trajectories, one can plot a collection of arrows representing the ``phase velocity" in phase space. This is not difficult to do for a two-droplet system with the help of constitutive relations. Particularly, assuming area conservation, i.e. $S_1+S_2=S_0$ with $S_0$ the total area determined by the initial condition, the trajectories are constrained within the line $S_2=S_0-S_1$. Similarly, the phase velocities are also parallel to this line, but can point either upward or downward. The constitutive relations can then be used to determine the direction of phase velocities at give $(S_1, S_2)$ by comparing the $S^*$ values corresponding to $S_1$ and $S_2$ respectively. Figure 2h shows the phase velocities determined following such procedure.

\subsection{Discussions on the structure of phase portrait}
As mentioned in the main text, one can immediately identify three different regions using the phase portrait in Fig. 2h, corresponding to three types of droplet behavior. In region I, all arrows point toward the equal-sized line $S_1=S_2$, indicating that the two droplets will exchange mass until they have equal sizes. In the language of dynamical systems, points on the line $S_1=S_2$ in region I are all stable fixed points. On the contrary, in region III, all arrays point away from the line $S_1=S_2$, a signature of unstable fixed points. Droplets with any initial sizes in this region will further differ in size until the smaller one is consumed by the other. Finally, as we go from region I to region II, points on the line $S_1=S_2$ transition from stable to unstable fixed points, but there are two branches of stable fixed points emerge (yellow solid lines), a typical manifest of supercritical bifurcation.

The overall structure of phase portrait can also be constructed by performing stability analysis of fixed points, as is usually done in dynamical systems. The first step is to find fixed points which, in our case, correspond to the states where the two droplets have fixed sizes or equivalently, equal values of $S^*$. In the case where two droplets are placed in identical vortices, they share a same $S-S^*$ curve. So the equal-sized states $S_1=S_2$ are always fixed points, as discussed earlier in this section. Since the $S-S^*$ curve has a nonmonotonic profile (see Fig. 2g), we can identify another branch of fixed points $S^*(S_1)=S^*(S_2)$ where $S_1$ and $S_2$ are in the regions of positive (negative) and negative (positive) slopes, respectively. This branch of fixed points is visualized by the orange solid lines in Fig. 2h. There are of course other fixed points which we will ignore at the moment. 

Let us now look at the stability of the equal-sized states. Consider a state $S_1=S_2$ and let us add a small perturbation $\delta S>0$ such that the areas become $S_1-\delta S$ and $S_2+\delta S$. The droplet will have completely different responses to this perturbation in the positive and negative slope regions. In the case of positive slope (regions II and III in Fig. 2h), the ECP decreases with increasing area. So, droplet 1 has a higher ECP than droplet 2, which will create a diffusive flux from droplet 1 to droplet 2 that further amplifies the area difference. Consequently, equal-sized states in the positive slope region is unstable as any perturbation can drive the system away from the fixed points. The story in the negative-slope region (region I in Fig. 2h) is the exact opposite. Here, the ECP actually increases with increasing area. Thus, the larger droplet, after the perturbation, has a higher ECP. A diffusive flux thus emerges that shrinks the larger droplet and brings the system back to the equal-sized state. These pictures can be clearly seen from the phase velocities in Fig. 2h.

The stability of the unequal-sized fixed points is slightly more complicated. Let us again consider a fixed point $S^*(S_1)=S^*(S_2)$ with $S_2>S_1$, and add a very small perturbation $\delta S>0$ such that the areas become $S_1-\delta S$ and $S_2+\delta S$. Using Taylor expansion, one can get $S^*(S_1-\delta S)\approx S^*(S_1)-\delta S\cdot dS^*(S_1)/dS$, $S^*(S_2+\delta S)\approx S^*(S_2)+\delta S\cdot dS^*(S_2)/dS$, and subsequently $\Delta S^*\equiv S^*(S_1-\delta S)-S^*(S_2+\delta S)\approx -dS\cdot[dS^*(S_2)/dS+dS^*(S_1)/dS]$. The stability of fixed points then depends on the slopes at $S_1$ and $S_2$. Note that $dS^*(S_2)/dS<0$ and $dS^*(S_1)/dS>0$, so  $\Delta S^* = dS\cdot[|dS^*(S_2)/dS|-|dS^*(S_1)/dS|]$. A stable fixed point requires droplet 1, after losing $\delta S$, to have a lower ECP. So, $\Delta S^*$ should be positive and $|dS^*(S_2)/dS|>|dS^*(S_1)/dS|$, meaning, the slope at $S_2$ should be steeper than that at $S_1$, which is true for the constitutive relations shown in Fig. 2g. This is why the unequal-sized branch is stable in Fig. 2h. 

Similar procedure can be done if the droplets are placed in vortices with different structures or speeds. Particularly, by simply changing the speed of vortices while keeping their overall structures, one can shift the position of fixed points, so the droplet sizes will be redistributed to coincide with the new stable fixed point. As illustrated in the main text, such mechanism can be used to tune the droplet sizes dynamically. For example, the red lines in Fig. 2i are obtained by switching the overall speeds $(v_{10}, v_{20})$ between $(3,5)$ and $(5,3)$. Consequently, the droplet sizes periodically swap between $(1613,1813)$ (green triangle in Fig. \ref{figS:PhasPort}b) and $(1813,1613)$ (orange triangle in Fig. \ref{figS:PhasPort}b).

\begin{figure}[h]
    \centering
    \includegraphics[width=1.0\textwidth]{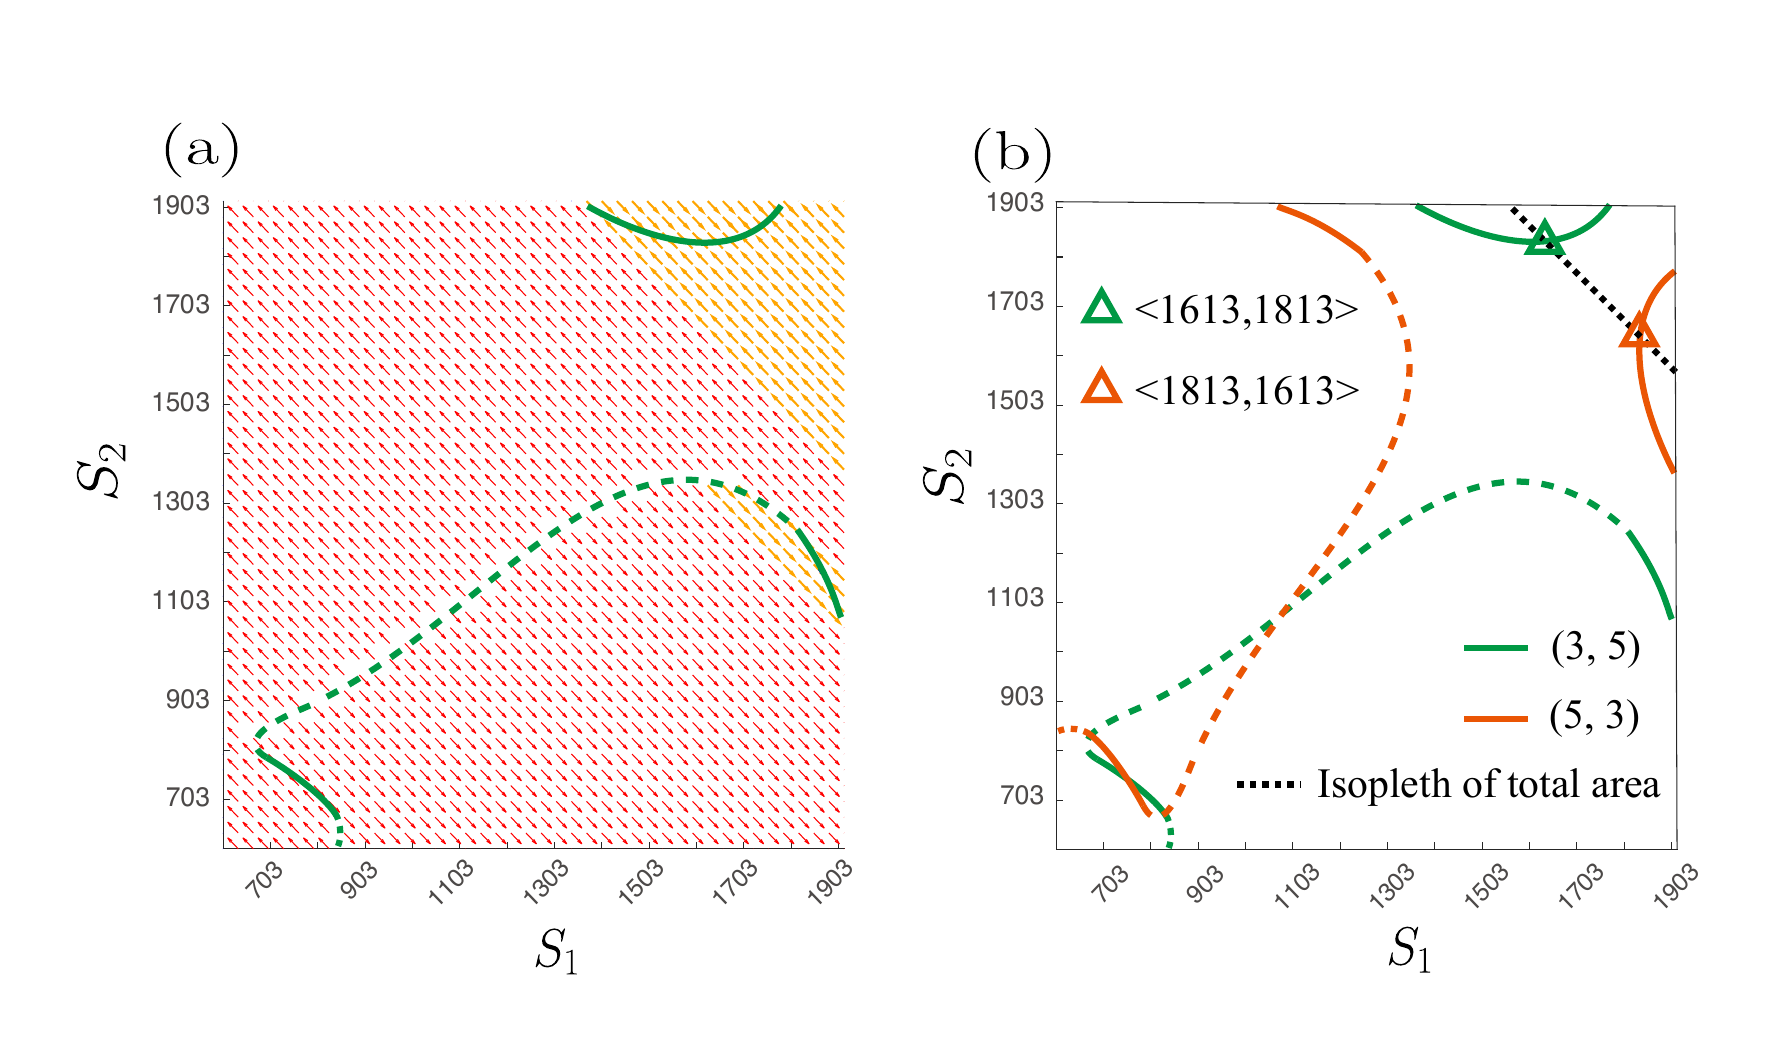}    
    \caption{(a) Phase two droplets placed in square vortices with different speeds: $v_{01}=3$ and $v_{02}=5$. The solid and dashed lines represent stable and unstable fixed points, respectively. (b) Fixed points of droplets at $(v_{01}=5,v_{02}=3)$ (green lines) and $(v_{01}=3,v_{02}=5)$ (orange lines).}
    \label{figS:PhasPort}
\end{figure}

% ----------------------------------------------
\section{Phase separation driven by vortex array and disordered flow}

This section provides extra results on phase separation driven by vortex array and disordered flows.

\subsection{Vortex array}
\begin{figure}[b]
    \centering
    \includegraphics[width=0.7\textwidth]{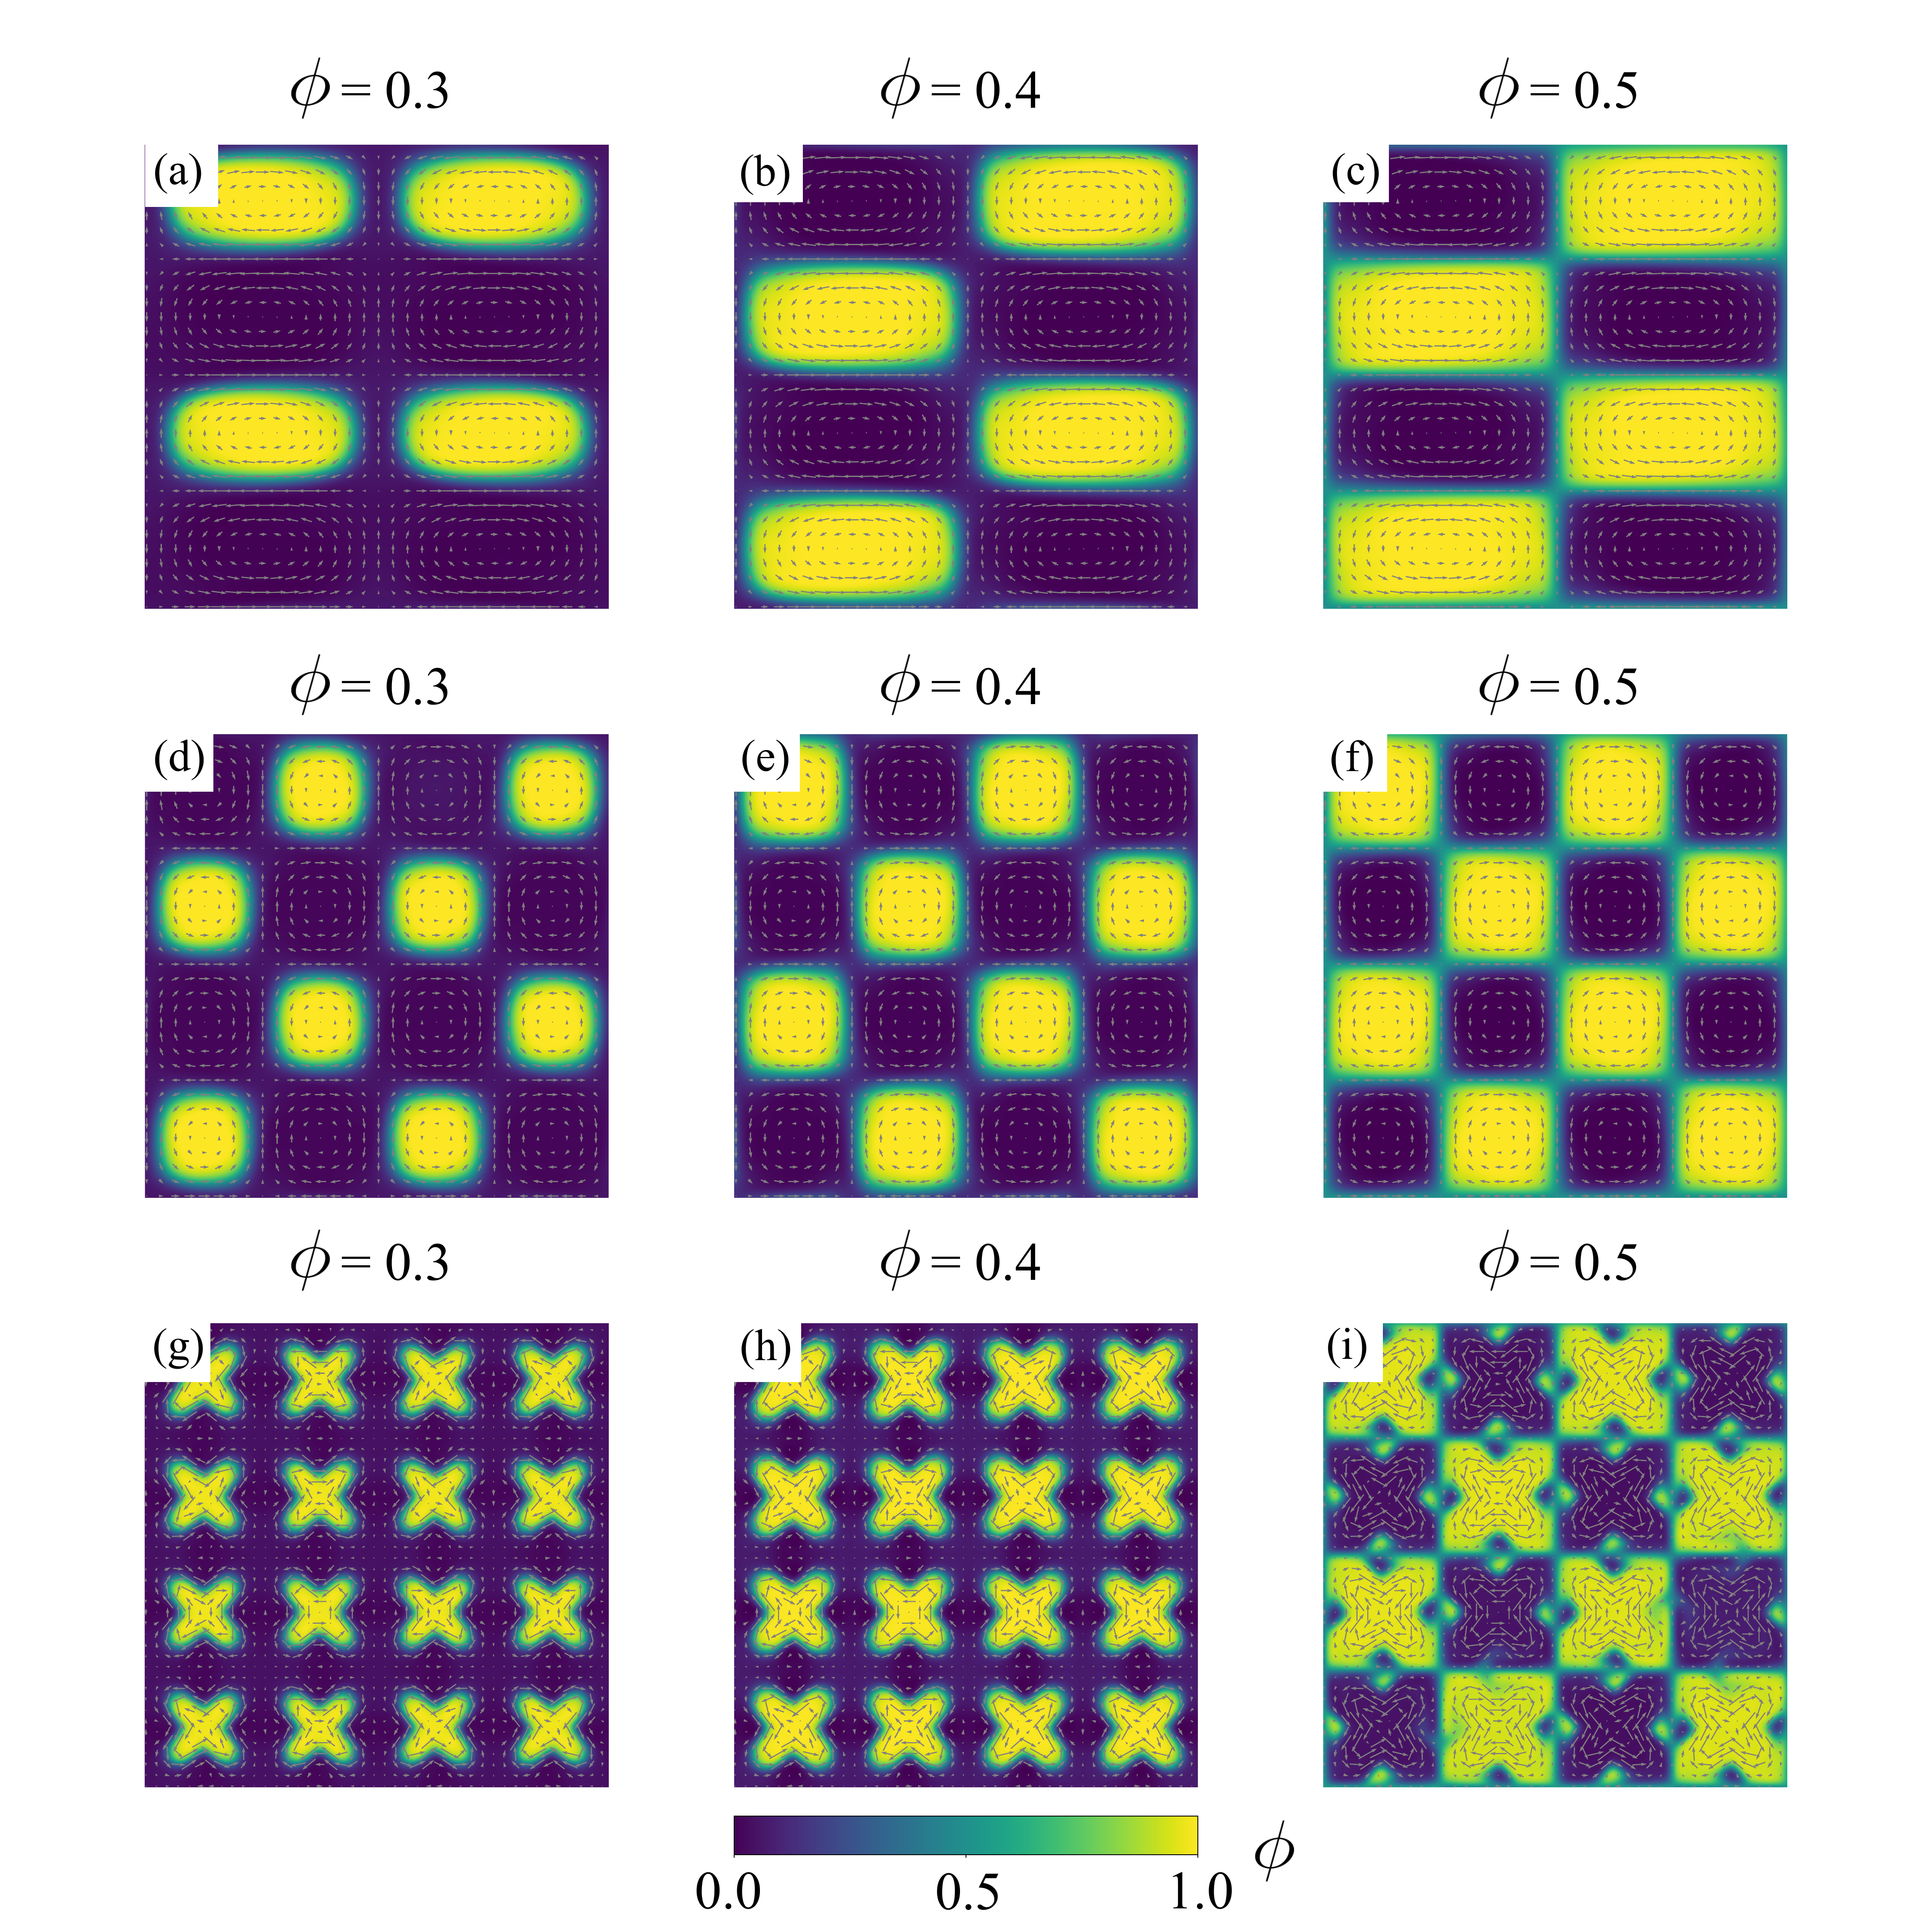}    
    \caption{Phase separation in vortex arrays with different initial compositions and flow structures.}
    \label{figS:lattice}
\end{figure}

As mentioned in the main text, periodic lattice of droplets can emerge from a phase separation driven by a vortex array. The specific structure of droplet lattice depends on the phase composition and the underlying vortex structure. Figure \ref{figS:lattice} shows the emergent structures at different conditions. Quite often, the droplets only occupy half of the vortices, which usually have the same direction of rotation (e.g. Figs. \ref{figS:lattice}b-\ref{figS:lattice}f). But there are also outliers such as Fig. \ref{figS:lattice}a, where vortices with different signs of vorticity contain droplets simultaneously. Most of the time, varying the composition $\phi_0$ does not alter the number of droplets, but changes the overall sizes of droplets instead. If the streamlines have negative curvature, droplets can only occupy part of the vortex, see Fig. \ref{figS:lattice}g-\ref{figS:lattice}h. In such case, full occupation is preferred. The exact behavior and the underlying mechanism are beyond the scope of this article.

\subsection{Disordered flow}

\begin{figure}[b]
    \centering
    \includegraphics[width=0.7\textwidth]{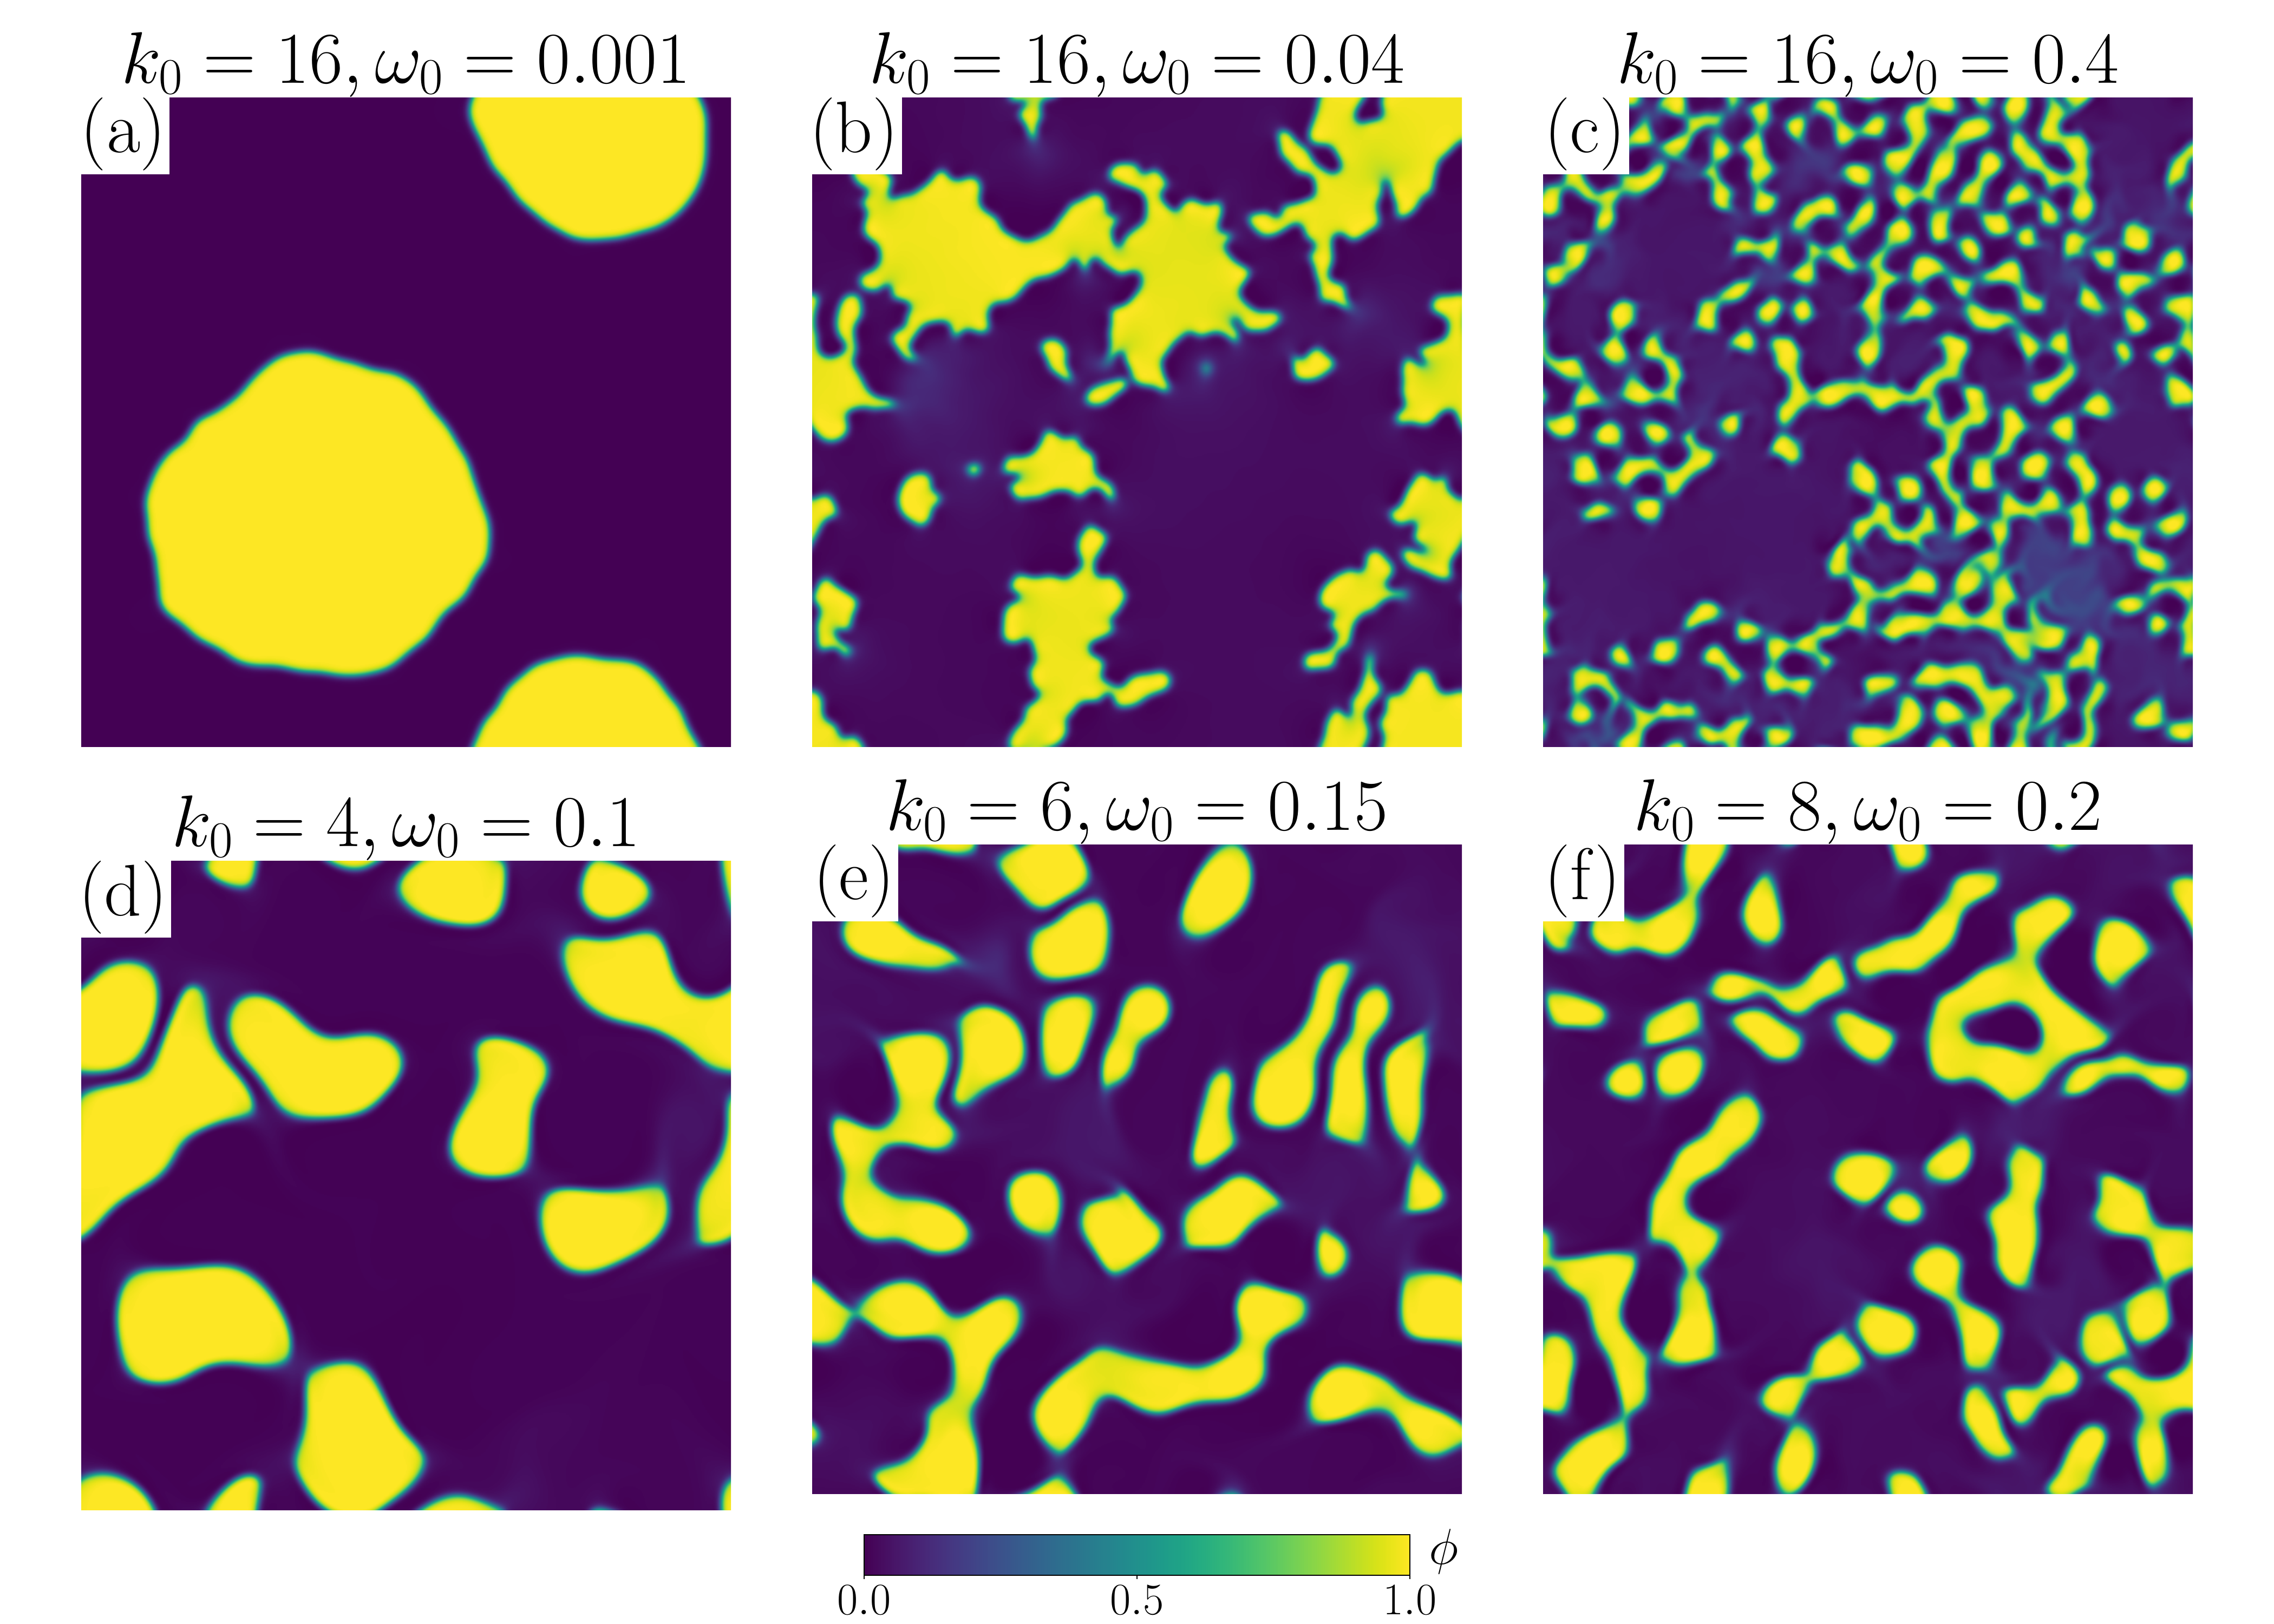}    
    \caption{Phase separation in disordered flow at different conditions.}
    \label{figS:disorder}
\end{figure}

Next, we investigate phase separation driven by flow fields with quenched disorder. To do this, we generate a random velocity field whose length scale is determined by a typical wavenumber $k_0$ and flow speed by a characteristic vorticity $\omega_0$. See Sec. 6C for details. Figure \ref{figS:disorder} shows the steady phase separated states driven by vortices with different speeds and length scales. It can be seen that a strong enough flow can arrest phase separation, giving a static phase field with a disordered structure, whose characteristic length is determined by that of the disordered flow.

% ----------------------------------------------
\section{Generation of different structured flow fields}

This section collects the specific numerical protocols to generate different types of structured flows used in this article. As mentioned in Sec. S1, the vortex-stream function method is used to generate the incompressible structured flow. Before that, we need to prescribe a velocity field that is simpler but does not necessarily satisfy the condition of incompressibility.

\subsection{Circular vortices in Fig. 1}

To generate a circular vortex, we first define a few parameters: the position of the vortex center $\textbf{r}_{c}$, the characteristic velocity $v_0$, and the radius of the vortex $r_0$. With these at hand, a circular vortex $\textbf{v}_0(\textbf{r})=[v_{0x}(\textbf{r}), v_{0y}(\textbf{r})]$ can be generated using $v_{0x}(\textbf{r}) = - \frac{\Delta y}{\Delta r} \times \frac{1}{2} v_0 (\Delta r/r_0)^n$ and $v_{0y}(\textbf{r}) = \frac{\Delta x}{\Delta r} \times \frac{1}{2} v_0 (\Delta r/r_0)^n$ if $\Delta r\le r_0$, and $v_{0x}(\textbf{r})=v_{0y}(\textbf{r})=0$ if $\Delta r> r_0$. Here, $\Delta r = |\textbf{r} - \textbf{r}_c|$ is the distance to the vortex center, and $\Delta x = (\textbf{r} - \textbf{r}_c)_x$, $\Delta y = (\textbf{r} - \textbf{r}_c)_y$. The parameter $n$ determines the radial dependence of velocity and angular velocity. In Fig. 1, we set $L_x=L_y=128$, $\textbf{r}_c=[L_x/2,L_y/2]$, $r_0 = L_x-10$. The values of $v_0$ and $n$ differ for different types of flow:
\begin{itemize}
\item Uniform angular velocity: $v_0 = 0.1$ and $n = 1$, giving $\Omega(r)=4.2 \times 10^{-5}$ (Vid. 1a);
\item Decreasing angular velocity: $v_0 = 0.02$, $n = 1/2$, giving $\Omega(r)=9.2 \times 10^{-5} r^{-1/2}$ (Blue line in Fig. 1c and Vid. 1b);
\item Increasing angular velocity: $v_0 = 0.1, n = 2$, giving $\Omega(r)=3.6 \times 10^{-6} r$ (Figs. 1a-1b, Orange line in Fig. 1c and Vid. 1c);
\item Increasing angular velocity: $v_0 = 0.2, n = 2$, giving $\Omega(r)=7.2 \times 10^{-6} r$ (Green line in Fig. 1c and Vid. 1d).
\end{itemize}

\subsection{Structured vortices in Fig. 2 and Fig. \ref{figS:PhasPort}}

The structured flows in Fig. 2 contain regions with active vortices and regions with nearly zero velocities. To generate $\textbf{v}_0$ for these structured flows, we divide the system into four equal-sized squares and assign $\textbf{v}_0$ values to each square independently.

For example, to generate the flow field in Fig. 2a in the main text, we set nonzero $\textbf{v}_0$ values to the lower-left square, while $\textbf{v}_0$ is zero in the other three squares. The lower-left square, containing a clover-shaped vortex, is assigned a velocity field: $v_{0x} = - v_1 \Delta y/\Delta r - k v_1 \sin(n \theta - \theta_c) \Delta x / \Delta r$ and $v_{0y} =  v_1 \Delta x/\Delta r - k v_1 \sin(n \theta - \theta_c) \Delta y/\Delta r$, where $v_1=v_0 \sin(\pi \Delta r / r_0)$. The first terms in $v_{0x}$ and $v_{0y}$ represent circular flow with rotational symmetry, while the second terms introduce anisotropy to the flow field with $k=2$ a coefficient used to adjust its relative weight. $n=4$ is the number of leaves, $\theta=\text{atan2}(\Delta y, \Delta x)$ and the rotation angle $\theta_c=0$. Similar to the circular flow, $\Delta r = |\textbf{r} - \textbf{r}_c|$, $\Delta x = (\textbf{r} - \textbf{r}_c)_x$, $\Delta y = (\textbf{r} - \textbf{r}_c)_y$. We set the vortex center $\textbf{r}_c=[L_x/4, L_y/4]$, vortex size $r_0=L_x/4$, and overall speed $v_0=1$. 

Such a flow field $\textbf{v}_0$, after enforced incompressibility, gives a relatively strong flow in the other three squares, which are supposed to have zero flow. So, the following iterative procedure is used to solve this problem:

\begin{itemize}
    \item Step 1: create a relatively simple flow field $\textbf{v}_0$ as mentioned above.
    \item Step 2: enforce the condition of incompressibility by using the vortex-stream function method, which gives a new flow field.
    \item Step 3: manually set the velocities in the other squares to be zero.
    \item Step 4: same as step 2.
    \item Repeat steps 3 and 4 until the velocities in the other squares are nearly zero.
\end{itemize}

Similar to Figs. 2a-2c, there is a single vortex in Fig. 2g. So the same procedure is used here, except that the clover-shaped vortex is replaced by a square vortex. The latter has the following flow field: $v_{0x} = -v_1 \Delta y/\Delta r + v_2 \Delta x/\Delta r \cdot \text{sign} (\text{mod}(n \theta, 2 \pi) - \pi) \cdot \cos{(n \theta)}$ and $v_{0y} = v_1 \cdot \Delta x/\Delta r + v_2 \cdot \Delta y/\Delta r \cdot \text{sign} (\text{mod}(n \theta, 2\pi) - \pi) \cdot \cos{(n \theta)}$. Here, $v_1=v_0 \cdot \sin{\pi \Delta r/r_0}$, $v_2=0.5 v_1 \cdot (\text{sign}(\Delta r-0.5 r_0)+1) \cdot \sin{((\text{sign}(\Delta r-0.5 r_0)+1)/2)}$ are the magnitudes of the isotropic and anisotropic components of the flow, respectively. $r_0$ is set to be $L_x/2$, and the overall speeds are: $v_0=1, 3, 5$ for the blue, red, orange lines.

In Figs. 2d-2f, 2h-2i, and \ref{figS:PhasPort}, the system contains two square vortices. So, we prescribe square vortices to the lower-left and top-right squares, while leaving the rest of the system flowless. The two square vortices only differ in the overall speed $v_0$. Once the initial flow field is assigned, we execute the iterative procedure mentioned before to enforce incompressibility and nearly zero flow in the top-left and lower-right squares.

\subsection{Structured vortices in Fig. 3, Fig. \ref{figS:lattice}, and Fig. \ref{figS:disorder}}

The flow fields in Figs. 3a-3c are similar to the circular vortices in Fig. 1 (see Sec. 6.A), but with different structure parameters. Specifically, we have $L_x=L_y=512$, and $v_0=1$ for Figs. 3a-3b. 

The procedure to generate vortex lattices depends on the specific lattice structure. To obtain the vortex lattice in Fig. 3d and Figs. S3g-3i, we divide the system into a 4x4 grid of squares. Then, in each square, we initiate a clover-shaped vortex (see Sec. 6.B), before enforcing incompressibility. The vortices in Fig. 3d and Figs. S3g-3i are identical, with the following parameters: $L_x=L_y=256$, $r_0=L_x/8$, $\theta_c=0$, $n=4$, $k=2$, and $v_0=1$.

The vortex lattices in Figs. S3a-3f are generated using a simpler method. Instead of generating the velocity field, we prescribe a periodic vorticity field $\omega(\textbf{r})$, and then use the vortex-stream function method to obtain the corresponding velocity field $\textbf{v}(\textbf{r})$. The vorticity field we used has the following form $\omega(x,y) = \omega_0 \cdot \sin{(2\pi k_xx/L_x)} \cdot \sin{(2\pi k_yy/L_y)}$, where $\omega_0$ represents the characteristic vorticity. $k_x$ and $k_y$ indicate the number of periods along the x and y direction respectively. The specific parameters are $\omega_0=1, k_x=1, k_y=2$ for simulations Figs. S3a-3c; and $\omega_0=1, k_x=2, k_y=2$ for simulations Figs. S3d-3e.

Generation of disordered flows in Figs. 3e-3f and \ref{figS:disorder} follows very similar procedure. We first generate a random vorticity field $\omega_1(x, y)$ where the value on each grid is randomly picked from a Normal distribution. This gives a field of random white noise without spatial structure. To create structures, we apply a wavenumber filter in Fourier space. Specifically, we Fourier transform $\omega_1(x, y)$ to get its Fourier amplitudes $\hat{\omega}_1(k_x, k_y)$, and filtering out the long-wave and short-wave components using $\hat{\omega}(k_x, k_y)=\hat{\omega}_1(k_x, k_y)\cdot F(|k|)$. $|k|=\sqrt{k_x^2+k_y^2}$ is the wavenumber and $F(|k|)=\omega_0 k_0^{4} \cdot k^{10}/(k_0^{14} + k^{14})$ is the filter with a characteristic wavenumber $k_0$ and a typical vorticity $\omega_0$. We then perform an inverse Fourier transform to get the vorticity field in real space $\omega(x,y)$.

The flow fields in Figs. 3g-3i are prescribed using the same method as the circular vortices, except that the initial flow structure takes the following form: $v_{0x} = -v_1 \Delta y/\Delta r + v_2 \Delta x/\Delta r \cdot \text{sign} (\text{mod}(n \theta, 2 \pi) - \pi) \cdot \cos{(n \theta)}$ and $v_{0y} = v_1 \cdot \Delta x/\Delta r + v_2 \cdot \Delta y/\Delta r \cdot \text{sign} (\text{mod}(n \theta, 2\pi) - \pi) \cdot \cos{(n \theta)}$. Again, $v_1=v_0 \cdot \sin{\pi \Delta r/r_0}$ and $v_2=0.5 v_0 \cdot (\text{sign}(\Delta r-0.5 r_0)+1) \cdot \sin{((\text{sign}(\Delta r-0.5 r_0)+1)/2)}$ are the magnitudes of the isotropic and anisotropic components of the flow, respectively. We set $n=2, r_0=L_x/2$. The flow speeds are $v_0=0.01$ for Fig. 3g, $v_0=1$ for Fig. 3h, and in Fig. 3i, $v_0$ varies from 0 to 10.

\subsection{Flows in Fig. \ref{figS:align}}

The flows in Figs. \ref{figS:align}a-\ref{figS:align}c have the same structure as the clover-shaped vortex in Fig. 2a, but differ in overall speed. Specifically, we have $v_0=0.001$ for Fig. S1a, $v_0=0.004$ for Fig. S1b and $v_0=0.1$ for Fig. S1c. 

The elliptical vortex in Fig. \ref{figS:align}d is generated using $v_{0x} = - v_0 \Delta y/b$ and $v_{0y} = v_0 \Delta x/a$, where $a$ and $b$ represent the major and minor axes of the ellipse, respectively. The parameters are $v_0=3, a=L_x/2, b=L_y/3$.

We generate the capsule-shaped vortex in Fig. \ref{figS:align}e by combining a rectangular flow field with two semicircular flow fields. To do this, we define two parameters: distance between the centers of the two semicircles $l_0$ and the radius of the semicircles $r_0$. The rectangular flow resides in the rectangular box $L_x/2-l_0/2\le x\le L_x/2+l_0/2$ and $L_y/2-r_0\le y\le L_y/2+r_0$. In this region, we set $v_x=-v_0 \cdot \sin{\pi \Delta y/r_0}, v_y=0$. Right next to the rectangular region, we have two semicircular flows attached to the left and right sides, respectively. The centers of the two semicircle are $[L_x/2-l_0/2, L_y/2]$ and $[L_x/2+l_0/2, L_y/2]$. In the semicircle, the velocity field is set as $v_x = -v \cdot \Delta y/r_0, v_y = v \cdot \Delta x/r_0$, where  $v=v_0 \cdot \sin{\pi \Delta r/r_0}$. The parameters used in Fig. S1e are $v_0=3$ and $r_0=L_x/4$.

Finally, the six-gear star in Fig. \ref{figS:align}f has the same expression of velocity as the vortices in Figs. \ref{figS:align}a-\ref{figS:align}c, but the structure parameters are slightly different: $n=6,v_0=3, k=2$ and $v_0 = 3$.

\newpage
\section{Videos}

\textbf{Vid. 1}: A single droplet in circular vortices with different angular velocities: (a) $\Omega(r)=4.2 \times 10^{-5}$, (b) $\Omega(r)=9.2 \times 10^{-5} r^{-1/2}$, (c) $\Omega(r)=3.6 \times 10^{-6} r$, and (d) $Omega(r)=7.2 \times 10^{-6} r$.

\textbf{Vid. 2}: Two droplets each driven by a patterned flow. (a) No flow in the background, corresponding to thermal equilibrium. (b-d) Corresponding to Figs. 2a, 2d, 2e in the main text, respectively.

\textbf{Vid. 3}: Dynamic manipulation of the droplet sizes. Panels a and b correspond to the blue and red lines in Fig. 2i in the main text.

\textbf{Vid. 4}: Phase separation (a) with and (b) without a structured flow in the background. Panel b corresponds to Fig. a in the main text.

\textbf{Vid. 5}: Phase separation driven by a periodic array of vortices, corresponding to Fig. 3d in the main text.

\textbf{Vid. 6}: Phase separation driven by a static disordered flow, corresponding to Fig. 3e in the main text.

\textbf{Vid. 7}: Melting of droplets by structured vortices. Panels a and b correspond to Figs. 3g and 3h in the main text. 

\textbf{Vid. 8}: Self-sustained oscillations of (a) a single droplet in a clover-shaped flow field with $v_0$ = 0.04, and (b) a lattice of droplets in a vortex array with initial $\phi_0=0.3$ and $\omega_0=0.1$.

\bibliographystyle{apsrev4-1}
% \bibliography{manipulating_LLPS_patterned_flow}
%
\end{document}
